# Supplementary material for: Negative Token Merging: Image-based Adversarial Feature Guidance
Source: arXiv:2412.01339 source file (2024-12-05)
Supplement: Supplementary file 1 [file X_suppl.tex]

\clearpage
\setcounter{page}{1}
\maketitlesupplementary

\appendix

\section{Additional Results and Applications}
\label{sec:applications}
%%% final list: additional applications
% improving output quality (done)
% subpart guidance
% image feature interpolation etc (done)
    % young old, 
% Style Variation.
    % bw sketch to colored sketch
% with controlnet (later if time)
% noisy to make it blur (reverse)
% better understanding diffusion manifold structure i.e. whats the first object when pushing away from something
In this section, we provide additional results and analysis which could not be included in the main paper due to space constraints. In particular, we provide results for following:
\begin{itemize}
    \item Results for complex and detailed prompts (Sec.~\ref{sec:complex-prompts})
    \item Generalization across diverse prompt styles (Sec.~\ref{sec:style-var})
    \item Analysis and results for grayscale outputs (Sec.~\ref{sec:bw})
    \item Additional results for improving diversity even when using prompt-rewriting using a LLM (Sec.~\ref{sec:pw})
    % \item Additional results for copyright mitigation (Sec.~\ref{sec:mitigation})
    \item Additional application: improving output aesthetics and details using a blurry reference (Sec.~\ref{sec:output-aesthetics}) 
    \item Additional application: object feature interpolation / extrapolation using a reference image (Sec.~\ref{sec:image-feat-interpolation})
    \item Cross-domain adversarial guidance: demonstrating the support for using of cross-domain images (\eg, sketch-to-photo) for adversarial guidance (Sec.~\ref{sec:crossdomain}) 
    % \item Uncurated results across different categories (Sec.~\ref{sec:uncurated-results}) 
\end{itemize}

% In this section, we provide additional results which could not be included in the main paper due to space constraints. In particular, we show results for generalization to complex / detailed prompts (Sec.~\ref{sec:complex-prompts}), generalization across diverse input prompt styles (Sec.~\ref{sec:style-var}), additional results for improving diversity when using prompt-rewriting (Sec.~\ref{sec:pw}), additional results for copyright mitigation (Sec.~\ref{sec:copyright}).
% Furthermore, we include results for additional applications of our approach such as improving output aesthetics (Sec.~\ref{sec:output-aesthetics}) and object feature interpolation / extrapolation (Sec.~\ref{sec:image-feat-interpolation}). Finally, we provide uncurated results for our method in Sec.~\ref{sec:uncurated-results}.

\subsection{Results for Complex / Detailed  Prompts}
\label{sec:complex-prompts}

We provide detailed results in Fig.~\ref{fig:complex-prompts-p1}, \ref{fig:complex-prompts-p2}. All prompts are randomly sampled using a large-language model \cite{achiam2023gpt} (\texttt{gpt-4o}), which is tasked to generated complex and detailed prompts for diverse output settings. We observe that using a complex / detailed prompt as the input actually worsens the limited diversity problem with the underlying base-model \cite{flux2024}.  This results in the output images displaying a limited variation in the output pose, scale, positioning, appearance of the different subjects. In contrast, by guiding the output image features away from each other during reverse diffusion process, the proposed approach helps significantly improve the output diversity across different attributes such as appearance, subject position, pose \etc.

For instance, in Fig.~\ref{fig:complex-prompts-p1}, we observe that when trying to generate an image of \bline{fisherman standing in calm river with a heron perched on rock nearby}, the base-model \cite{flux2024} results in limited variation in overall scene appearance, subject position,  and scale of different subjects. In contrast, NegToMe is able to better harness the inner diversity of the diffusion model resulting in outputs with varying positions / scales for both \bline{fisherman} and \bline{heron}. Also the resulting appearances for both subjects (\emph{color of jacket, hat, clothing, color of bird \etc}) are more diverse. Additionally, the overall appearance and other global  background features (\eg, misty appearance, time of day, color of water, background \etc) also show better diversity when using the proposed approach (while still just using $<4\%$ higher inference times).

Similarly, in Fig.~\ref{fig:complex-prompts-p2}, when generating an image for \bline{a knight surfing on vibrant blue waves}, we observe that the base-model \cite{flux2024} results in limited variation in position of the main subject (\bline{knight}), subject scale and size, color of waves, flowers \etc. In contrast, NegToMe helps significantly improve the output diversity in terms of position and scale of the main subject (\bline{knight}). Furthermore, the overall appearance and background features such as color of waves, flowers \etc also shows much higher output diversity.
% as opposed to the base-model (while still just using $<4\%$ higher inference times).

\begin{figure*}[htbp]
\vskip -0.3in
\begin{center}
% \centerline{\includegraphics[width=1.\linewidth]{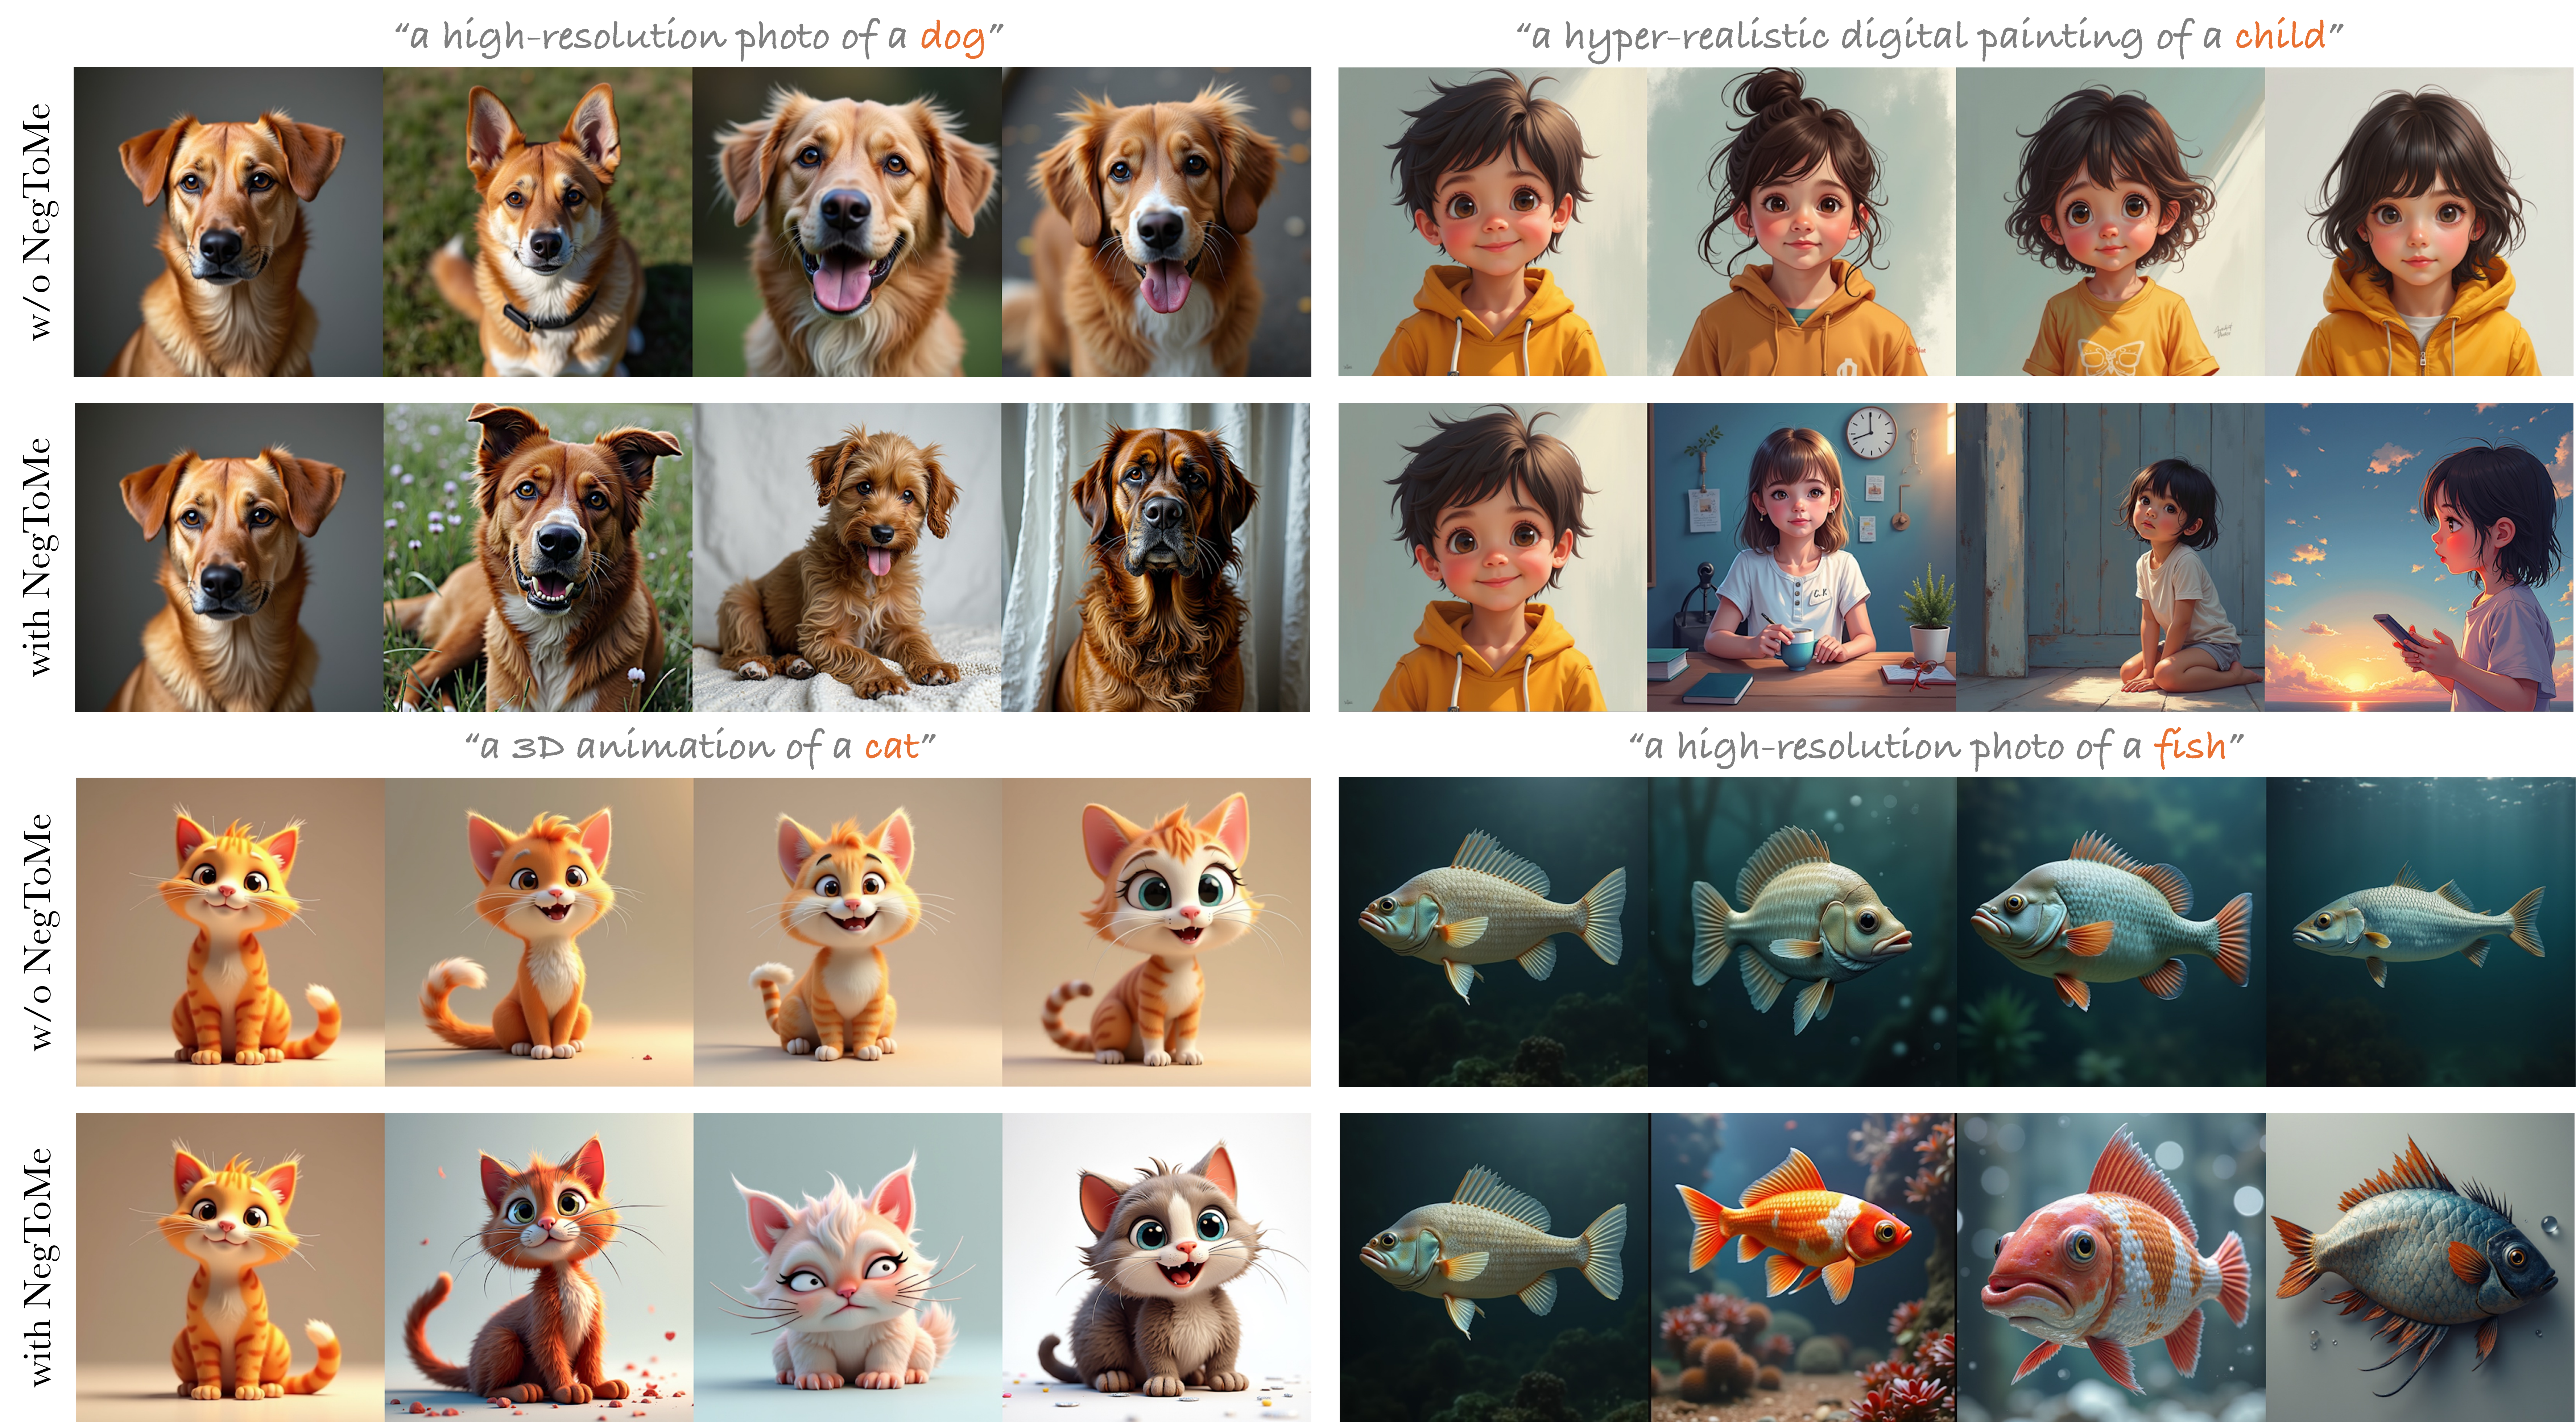}}
\centering
     \begin{subfigure}[b]{0.94\textwidth}
         \centering
         \includegraphics[width=1.\textwidth]{assets/complex-prompt-p1-v1.pdf}
         % \caption{\emph{Success case}}
         % \label{fig:var-domain}
     \end{subfigure}
     % \vskip 0.1in
     \begin{subfigure}[b]{0.94\textwidth}
         \centering
         \includegraphics[width=1.\textwidth]{assets/complex-prompt-p2-v1.pdf}
         % \caption{\emph{Success case}}
         % \label{fig:var-domain}
     \end{subfigure}
     % \vskip 0.1in
     \begin{subfigure}[b]{0.94\textwidth}
         \centering
         \includegraphics[width=1.\textwidth]{assets/complex-prompt-p3-v1.pdf}
         % \caption{\emph{Success case}}
         % \label{fig:var-domain}
     \end{subfigure}
% \vskip -0.15in
\caption{\emph{\textbf{Results for complex prompts.} } NegToMe works across prompts of different complexity and detail. Above we see it improves output diversity for different image attributes such as subject appearance (\eg, \emph{elemental creature, fisherman}), subject pose and scale (\eg, \emph{fisherman, wizard}), subject position (\emph{wizard}), as well as overall background appearance (\emph{time-of-day, color of river, color of portal}) \etc.}
\label{fig:complex-prompts-p1}
\end{center}
\vskip -0.2in
\end{figure*}

\begin{figure*}[htbp]
\vskip -0.3in
\begin{center}
% \centerline{\includegraphics[width=1.\linewidth]{assets/flux-diversity-v1.pdf}}
\centering
     \begin{subfigure}[b]{0.94\textwidth}
         \centering
         \includegraphics[width=\textwidth]{assets/complex-prompt-p4-v1.pdf}
         % \caption{\emph{Success case}}
         % \label{fig:var-domain}
     \end{subfigure}
     % \vskip 0.1in
     \begin{subfigure}[b]{0.94\textwidth}
         \centering
         \includegraphics[width=1.\textwidth]{assets/complex-prompt-p5-v1.pdf}
         % \caption{\emph{Success case}}
         % \label{fig:var-domain}
     \end{subfigure}
     % \vskip 0.1in
     \begin{subfigure}[b]{0.94\textwidth}
         \centering
         \includegraphics[width=1.\textwidth]{assets/complex-prompt-p6-v1.pdf}
         % \caption{\emph{Success case}}
         % \label{fig:var-domain}
     \end{subfigure}
% \vskip -0.15in
\caption{\emph{\textbf{Results for complex prompts.}} NegToMe works across prompts of different complexity and detail. Above we see it improves output diversity for different image attributes such as subject age and appearance (\eg \emph{panda}), subject pose and scale (\eg \emph{dog, knight}), subject position (\emph{knight}), as well as overall background appearance (\eg \emph{time-of-day, color of river, style of woven-hat}) \etc}
\label{fig:complex-prompts-p2}
\end{center}
\vskip -0.2in
\end{figure*}

\subsection{Generalization across Style Variation}
\label{sec:style-var}

We next provide results analyzing the generalization of the proposed approach across different input styles (\emph{\eg watercolor, photo, 3D animation, japanese anime \etc}). Results are shown in Fig.~\ref{fig:style-var}, \ref{fig:style-var2}. To demonstrate the practical usefulness of our approach, all prompts are sampled randomly using a large-language model \cite{achiam2023gpt} (\texttt{gpt-4o}), which is tasked to detailed prompts for diverse output settings. 

As seen in Fig.~\ref{fig:style-var}, \ref{fig:style-var2} we observe that the base model often shows limited diversity across the output generations even when scaling across diverse output styles (\emph{\eg watercolor, photo, 3D animation, japanese anime \etc}). For instance, when generating an image of a \bline{deer standing in an open meadow}, the base-modal shows limited variations in the appearance of the dear as well as the background. Similarly, when generating a \bline{couple walking hand in hand along a tree-lined misty park}, the base model \cite{flux2024} generated virtually same outputs in terms of scene appearance, time of day, position and scale of the subjects \etc.

The proposed approach is able to address the above problems, thereby improving the output diversity across diverse visual attributes. For instance, for the image of \bline{couple walking hand in hand along a tree-lined misty park}, we observe that it helps improve output diversity across position and scale of the \emph{couple}, overall scene appearance / lighting, background attributes such as direction of the \emph{tree-line path}, color of trees \etc. Similarly, in Fig.~\ref{fig:style-var2}, we observe that it helps improve diversity for the appearance of the background \emph{meadow},  pose and scale of the main subject (\emph{dear}), time-of-day (sunset, daytime \etc) in the resulting images.

\begin{figure*}[t]
% \vskip -0.15in
\begin{center}
% \centerline{\includegraphics[width=1.\linewidth]{assets/flux-diversity-v1.pdf}}
\centering
     \begin{subfigure}[b]{0.95\textwidth}
         \centering
         \includegraphics[width=1.\textwidth]{assets/style-var-p1-v3.pdf}
         % \caption{\emph{Success case}}
         % \label{fig:var-domain}
     \end{subfigure}
     % \vskip 0.1in
     \begin{subfigure}[b]{0.95\textwidth}
         \centering
         \includegraphics[width=1.\textwidth]{assets/style-var-p2-v1.pdf}
         % \caption{\emph{Failure case}}
         % \label{fig:var-ngrad}
     \end{subfigure} 
\vskip -0.15in
\caption{\emph{\textbf{Generalization across different styles.}} We observe that NegToMe generalizes and increases output diversity across different style variations in the input prompt. All results are reported with fixed seed $\leftarrow$ 0. Furthermore, to practical useful across diverse prompts, we use generic detailed prompts which are sampled using \texttt{gpt-4o}. NegToMe improves output diversity across several attributes such as subject scale and position (\emph{child, couple}), as well as overall scene appearance (\eg, time-of-day, direction of road, color of trees \etc)}
\label{fig:style-var}
\end{center}
\vskip -0.2in
\end{figure*}

\begin{figure*}[t]
% \vskip -0.15in
\begin{center}
\centerline{\includegraphics[width=1.\linewidth]{assets/style-var-p3-v1.pdf}}
\vskip -0.1in
\caption{\emph{\textbf{Generalization across different styles.}} We observe that NegToMe generalizes and increases output diversity across different style variations in the input prompt. All results are reported with fixed seed $\leftarrow$ 0. Furthermore, to practical useful across diverse prompts, we use generic detailed prompts which are sampled using \texttt{gpt-4o}. We see that NegToMe improves output diversity across several attributes such as subject scale and appearance (\emph{dear}), as well as overall scene appearance (\eg, time-of-day, color of meadow \etc)}
\label{fig:style-var}
% \caption{\emph{\textbf{Generalization across different styles.}} We observe that NegToMe generalizes and increases output diversity across different style variations in the input prompt. All results are reported with fixed seed $\leftarrow$ 0. Furthermore, to demonstrate the generalization across diverse prompts, we use generic detailed prompts which are sampled using \texttt{gpt-4o}.}
\label{fig:style-var2}
\end{center}
% \vskip -0.3in
\end{figure*}

\subsection{Results for Grayscale Outputs}
\label{sec:bw}

\begin{figure*}[t]
% \vskip -0.15in
\begin{center}
\centerline{\includegraphics[width=1.\linewidth]{assets/bw-diversity-v1.pdf}}
\vskip -0.1in
% \caption{\emph{\text{NegToMe with prompt-rewriting (PW).}}}
\caption{\emph{\textbf{Does NegToMe work for grayscale images?}} We observe that NegToMe leads to improved output diversity (\eg species for animal; gender, age for peron; pose, appearance for cat, fish \etc)  even when constrained to grayscale image outputs.}
\label{fig:bw-results}
\end{center}
% \vskip -0.3in
\end{figure*}

In order to fully understand the ability of the proposed approach for promoting semantic feature diversity, we also analyze the performance of our approach when limited to grayscale outputs (\eg, \emph{black and white photo}). Since the outputs are constrained to be grayscale, increased diversity can only be obtained by increasing the variation along other semantic attributes such as \emph{gender, age} for humans, \emph{pose, scale, species, appearance} for general objects \etc (Fig.~\ref{fig:bw-results}).

Results are shown in Fig.~\ref{fig:bw-results}. We observe that even when constrained to grayscale image outputs (using the prompt template: \emph{`a black and white photo of'}, \negtome~significantly increases the output diversity across other meaningful semantic attributes. For instance, when generating a \bline{black and white photo of an animal}, the base-model \cite{flux2024} leads to outputs which predominantly resemble a \emph{wolf} and show appearance similarities across generations. In contrast,  the proposed approach is able to significantly improve diversity leading to different animals such as \emph{wolf, goat, baby-bear, horse} leading to better output diversity. 

Similarly, when generating a \bline{black and white photo of a person}, we observe that the base-model \cite{flux2024}, only generates female outputs. The application of \negtome~ not only helps improve the gender diversity (generating both male and female), but also increases the variance along the age axis, outputting an image of a young child (col-2: Fig.~\ref{fig:bw-results}).

\subsection{Additional Results with Prompt-Rewriting.}
\label{sec:pw}

A key advantage of \negtome is that it helps improve diversity without the need for extensive prompt-rewriting, which also presents as a feasible yet expensive (time \& memory) approach for improving diversity. This is particularly relevant when the user-prompts are quite detailed and long. We next demonstrate that NegToMe helps improve output diversity both with and without prompt-rewriting.
For each prompt, prompt-rewriting is performed by using a large-language model (\texttt{gpt-4o}) \cite{achiam2023gpt} in order to generate diverse variations of the original base prompt.

% To provide a fair comparison with prompt-rewriting setting, we therefore first curate a set of 20 detailed prompts across diverse settings (see appendix). For each prompt we then use a large-language model \cite{achiam2023gpt} in order to generate diverse variations of the original base prompt. The final images for both base-prompt and rewritten prompts are sampled across 10 random seeds.
% % Finally, we sample 10 images per random seeds
% % We compare with prompt-rewriting based on FLUX in Fig.~\ref{fig:prompt-rewriting}.
% % and Tab.~\ref{tab:prompt-rewriting}. 

Results are shown in Fig.~\ref{fig:prompt-rewriting} (in addition to quantitative results from Sec.~\ref{sec:output-diversity} of main paper).
While prompt-rewriting helps improve diversity, it comes at the cost of increased inference time. Furthermore, some of the generated outputs might still appear similar (\eg, col-1 and col-3 for cat: Fig.~\ref{fig:prompt-rewriting}). In contrast, \negtome can adaptively improve the output diversity (with both base and rewritten prompts), while on average using only $<4\%$ higher inferences times (see Sec.~\ref{sec:output-diversity} of main paper for detailed quantitative results).

\begin{figure*}[t]
% \vskip -0.15in
\begin{center}
% \centerline{\includegraphics[width=1.\linewidth]{assets/flux-diversity-v1.pdf}}
\centering
     \begin{subfigure}[b]{0.51\textwidth}
         \centering
         \includegraphics[width=1.\textwidth]{assets/pw-p1-v1.pdf}
         % \caption{\emph{Success case}}
         % \label{fig:var-domain}
     \end{subfigure}
     % \vskip 0.1in
      \begin{subfigure}[b]{0.475\textwidth}
         \centering
         \includegraphics[width=1.\textwidth]{assets/pw-p2-v1.pdf}
         % \caption{\emph{Success case}}
         % \label{fig:var-domain}
     \end{subfigure}
% \vskip -0.15in
\caption{\emph{\textbf{NegToMe with Prompt-rewriting.}} We observe that NegToMe helps improve output diversity both without (row-2: size of ball, pose of cat, panda) and with explicit prompt-rewriting (PW) (row-4: size, pose of cat and panda).}
\label{fig:prompt-rewriting}
\end{center}
\vskip -0.2in
\end{figure*}

% \begin{figure}[t]
% % \vskip -0.15in
% \begin{center}
% \centerline{\includegraphics[width=0.9\linewidth]{assets/prompt-rewriting-v2.pdf}}
% \vskip -0.1in
% % \caption{\emph{\text{NegToMe with prompt-rewriting (PW).}}}
% \caption{NegToMe helps improve output diversity both with (row-2) and without explicit prompt-rewriting (PW) (row-4).}
% \label{fig:prompt-rewriting}
% \end{center}
% % \vskip -0.3in
% \end{figure}

% \subsection{Additional Results for Copyright Mitigation.}
% \label{sec:mitigation}

\subsection{Improving Output Aesthetics.}
\label{sec:output-aesthetics}

\begin{figure}[t]
\vskip -0.15in
\begin{center}
\centerline{\includegraphics[width=1.\linewidth]{assets/output-quality-p2-v1.pdf}}
\vskip -0.1in
\caption{\emph{\textbf{Improving output aesthetics.}} We find that using a blurry or poor quality reference with NegToMe helps improve output aesthetics and details. Best viewed zoomed-in.}
\label{fig:output-quality}
\end{center}
\vskip -0.1in
\end{figure}

We also provide further results for some additional applications of the proposed approach. Interestingly, as noted in Sec.~\ref{sec:analysis}, we find that when performing adversarial guidance with a poor quality and blurry image \negtome~leads to improved output aesthetics and details. Importantly, such improvements are observed even when using \emph{state-of-the-art} diffusion models such as Flux-Dev \cite{flux2024}, which have already been guidance-distilled in order to obtain high image quality (without the need to adjust the negative prompt).

Results are shown in Fig.~\ref{fig:output-aesthetics}. We observe that simply using a blurred reference image with \negtome~leads to improved output aesthetics and level of details in the generated image outputs. For instance, when generating a \bline{painting of a woman}, the base Flux model \cite{flux2024} leads to almost photo-realistic image outputs with limited artistic style. The use of the proposed approach with a blurry reference helps address this issue, generating output images with better aesthetic details (\eg, lighting, color of the painting) while also  improving the level of artistic details in generated painting. 

Similarly, as seen in Fig.~\ref{fig:output-aesthetics}, when generating a \bline{photo of a bird}, we observe that the generated images exhibit limited output details for the both the main subject as well as the background.  The use of the proposed approach helps address this problem by gradually increasing the level of detail in both the main subject (\eg head of bird) as well as the background (\eg, tree branch \etc).

\subsection{Image feature Interpolation.}
\label{sec:image-feat-interpolation}

We next explore another application of the proposed approach for object feature interpolation or extrapolation using a reference image. 
The interpolation and extrapolation are simply achieved by either guiding the output image towards or away from the reference image using NegToMe. 

Results are shown in Fig.~\ref{fig:feature-interpolation}. We observe that the proposed approach allows for a range of diverse object feature interpolations using a reference image. For instance, given an input prompt \bline{an animal} and original image of a \emph{deer}, we can guide the generated image either towards or away from features of the provided reference image (\emph{tiger} in Fig.~\ref{fig:feature-interpolation}). Interestingly, pulling the \emph{deer} features closer to \emph{tiger} first results in a \emph{fox} before finally transitioning to the appearance of the reference (\emph{tiger}). On the other hand, \negtome~can also be used to push the output features away from those of the \emph{tiger}, which leads to the output animal becoming more cuter and less scary transitioning from a \emph{baby dear} to a \emph{cute dog like animal}.

Similarly, when using an original image of a \emph{young cat} and performing feature interpolation / extrapolation using an image of a \emph{kitten}, we observe that \negtome allows for interpolation for the age and appearance related features.  For instance, when pulling the features closer to that of the kitten we observe that the original cat appears to become smaller and younger. On the other hand, pushing the output features away from that of the \emph{kitten} leads to the output \emph{cat} become larger and older (see Fig.~\ref{fig:feature-interpolation} for further results).

\subsection{Cross-domain Adversarial Guidance}
\label{sec:crossdomain}
% \noindent\emph{\textbf{Cross-domain feature guidance.}}
% \noindent\emph{\textbf{Does NegToMe work with cross-domain reference?}}
% sketch to photo / painting e.g. dog species example in slides
 
We also explore the robustness of our approach to performing adversarial guidance when the provided reference image (\eg, sketch) is from a different style / modality as compared to the desired output image (\eg, photo). 

Results are shown in Fig.~\ref{fig:cross-domain-var}. We observe NegToMe can also be used even when even when the provided reference image has a different style and pose \emph{w.r.t} to desired outputs (\eg, sketch of dog in Fig.~\ref{fig:cross-domain-var}). This happens due to the use of  
the (semantic) token matching step (refer Sec.~\ref{sec:method} of main paper) which only matches each token with other tokens with similar attribute semantics.
% with NegToMe allows for feature guidance across object features, appearance \etc.

Similarly, even when using a water-color illustration of a jeep as reference, the proposed approach allows for performing adversarial guidance by only matching the relevant features of the jeep and pushing them away during the reverse diffusion process. This leads to the output \emph{vehicle} gradually moving away from the features of the \emph{jeep} and moving towards \emph{car} (see Fig.~\ref{fig:cross-domain-var} for further results).
 
 % As shown in Fig.~\ref{fig:cross-domain-var}, we find that even when the provided reference image has a different style and pose \emph{w.r.t} to desired outputs, the semantic token matching step (Sec.~\ref{sec:method}) with NegToMe allows for feature guidance across object features, appearance \etc.

\begin{figure}[t]
\vskip -0.15in
\begin{center}
\centerline{\includegraphics[width=1.\linewidth]{assets/cross-domain-v2.pdf}}
\vskip -0.1in
\caption{\emph{\textbf{Cross-domain feature guidance.}} NegToMe can also be used across-domains (\eg, sketch-photo above) in order to push the output features away from the concepts in the reference image.}
\label{fig:cross-domain-var}
\end{center}
\vskip -0.1in
\end{figure}

\begin{figure*}[htbp]
\vskip -0.15in
\begin{center}
\centerline{\includegraphics[width=1.\linewidth]{assets/feature-interpolation-v1.pdf}}
\vskip -0.1in
\caption{\emph{\textbf{Additional Application: Object feature interpolation.}} We observe that NegToMe also enables additional applications such as object feature interpolation (by guiding the output features towards the reference using $\alpha < 0$) and extrapolation (by guiding the output features away from the reference using $\alpha > 0$).  For instance, pulling a \emph{young cat (row-2)} towards the features of a \emph{kitten} for makes the output cat smaller and younger. On the other hand, guiding it away from visual features of the \emph{kitten} makes it older and bigger.}
\label{fig:feature-interpolation}
\end{center}
\vskip -0.1in
\end{figure*}

\section{Additional Experiment Details}
\label{sec:experiment details}
% experiment details for different experiments
% prompts, user study, other things referenced in the main paper
% PW prompt etc
 
 % \emph{\textbf{Implementation Details.}} \lipsum[1]
% we implement using open-source SDXL models and Flux for MMDiT. all results are reported using 1024x1024 on a single Nvidia-H100 GPU. 
% We use publicly available 

\subsection{Implementation Details.}
% different hyperparams
% take the paragraph from main paper
% difference for SDXL and Flux
% how many steps, alpha, threshold

\textbf{Model Details.} We use publicly available open-source models for implementing our approach (Sec.~\ref{sec:method}). In particular, we use SDXL \cite{podell2023sdxl} for implementation on UNet based diffusion models. Guidance distilled Flux-Dev \cite{flux2024} is used for implementing on MM-DiT style joint-attention models. Unless otherwise specified, all results are reported at 1024x1024 on a single Nvidia-H100 GPU. 

\noindent\textbf{Applying NegToMe in transformer block.} The NegToMe module (Alg.~\ref{alg:negtome} of main paper) is inserted after the attention layer in each transformer block of the diffusion model. For SDXL we primarily apply the negative token merging module in the up-blocks of the UNet model. For Flux, we apply negative token merging across the joint-attention blocks in the MM-DiT model. While we do observe that we can reduce inference time costs by applying NegToMe 
only in the last $M \in [20, 30]$ transformer blocks of the MM-DiT model, for simplicity and ease of implementation we apply NegToMe across all joint attention blocks with Flux \cite{flux2024}.

\noindent \textbf{Hyperparamters.} To minimize additional inference costs we find that applying NegToMe only in the initial part of the reverse diffusion process is sufficient for obtaining adversarial guidance \emph{w.r.t} key image features. 
We therefore limit the application of NegToMe for first $t \in [1000, 600]$ timesteps for SDXL \cite{podell2023sdxl}, and $t \in [1000, 900]$ for Flux \cite{flux2024}. A threshold $\tau=0.7$ is used for semantic token matching (Sec.~\ref{sec:method} ) to avoid \emph{source} tokens with no good semantic match to be changed during negative token merging.  

% \textbf{Hyperparameters.}

\subsection{Quantitative Experiments}

% \textbf{Output Diversity Experiments}
% prompt templates
% prompt for gpt4o for PW
% prompt

\textbf{Increasing Output Diversity.}
We evaluate the performance of our approach for increasing output diversity when performing negative token merging \emph{w.r.t} 
to other images in the batch. To facilitate easy visual comparison, we perform negative token merging \emph{w.r.t} 
the first image in each batch while reporting results in the paper. 

For evaluation, we first construct an input prompt dataset comprising 20 general object categories across 7 different prompt templates (\eg, ``a photo of a'', ``a high-contrast image of a''). The prompt templates are adopted from the CLIP prompt templates~\cite{radford2021learning} for CIFAR10 image classification, excluding ones that imply low-quality (\eg, \emph{``a blurry photo of a''}). For object categories, we use random generic categories \emph{['animal', 'bird', 'mammal', 'person', 'man', 'woman', 'child', 'dog', 'cat', 'boat', 'building', 'bus', 'car', 'airplane', 'fish', 'bridge', 'insect/bug', 'snake', 'shirt', 'dress']}  for exhibiting the generalization of our approach across diverse settings and subjects.

For each category, we sample 280 images with 10 random seeds (4 per batch) both with and without \negtome. The real images for FID \cite{heusel2017gans} calculation are sourced from LAION-Aesthetics-v2 6+ dataset \cite{schuhmann2021laion}, where we use  CLIP~\cite{radford2021learning} to retrieve the top-1K images for each category.

% measures the degree to which outputs for a particular object category (\eg, person) are spread across its subcategories (racial, gender, ethnic \etc). 

In addition to using pairwise Dreamsim-Score \cite{fu2023dreamsim} for measuring diversity, we also use an Entropy-Score \cite{elgammal2017can} which measures the degree to which outputs for a particular object category (\eg, person) are spread across its subcategories (racial, gender, ethnic \etc). 
 1) For a given general non-human category (\eg, `bird'), we first extract possible sub-categories (\eg, `sparrow', `eagle') using WordNet~\cite{miller1995wordnet}. Next, we classify the generated images into one of these sub-categories by leveraging CLIP image-text similarity, using the standard zero-shot ImageNet classification prompt template described in~\cite{radford2021learning}. 2) For generated human images, we follow~\cite{Wan2024TheFT} to use the pre-trained FairFace classifier~\cite{Krkkinen2019FairFaceFA} to identify demographic traits, including race, gender, and age. The diversity for each category is quantified using the entropy $\mathcal{E}$ of the resulting distribution as $\mathcal{E} = -\sum_{i=1}^n p_i \log p_i$, where \( p_i \) is proportion of images classified into sub-category \( i \), and \( n \) is total number of sub-categories. The final entropy-score is computed as average across all considered categories (refer Sec.~\ref{sec:experiments} for results).

% \noindent 
\textbf{Copyright mitigation.}
We also show the efficacy of our approach for reducing visual similarities with copyrighted characters when performing negative token merging \emph{w.r.t} a copyrighted image RAG database (Sec.~\ref{sec:copyright}). 

The copyrighted RAG database consists 50 copyrighted characters (\eg, Mario, Elsa, Batman, Yoda \etc), and includes input prompts which trigger these characters without explicitly mentioning their names. For each character, we compile a reference dataset of approximately 30 high-quality images depicting the character in diverse settings. The RAG assets for each character include a combination of real character images (scraped from the internet) as well as high quality generated images (which are manually filtered to ensure representation of desired character). The mask for each asset is computed using HQ-SAM \cite{sam_hq}.

For evaluation, we use the Dreasim-score, reporting the maximum similarity of the generated images (with and without NegToMe) across all copyrighted images in the dataset (excluding the one used for NegToMe guidance). Following the original paper \cite{fu2023dreamsim}, we adopt the background removal strategy in order to ensure that the final results only indicate the similarity with respect to the copyrighted characters and are not affected by background features. 

\begin{figure*}[htbp]
\vskip -0.15in
\begin{center}
\centerline{\includegraphics[width=1.\linewidth]{assets/copyright-full-prompt-v1.pdf}}
\vskip -0.1in
\caption{Copyright mitigation results with complete prompts for Fig.~\ref{fig:copyright-qual} in main paper.}
\label{fig:copyright-complete-prompt}
\end{center}
\vskip -0.1in
\end{figure*}

% \lipsum[1]

% complete prompts 
% character names

% \textbf{User-Study.}

%-------------------------------------------------------------------------
% \newpage
\section{Discussion and Limitations}
\label{sec:limitations}
% lack of disentanglement with different features pose, lighting etc.
% while masked guidance provides an avenue for such control, Furthermore combining it with text adversarial guidance also improve scontrol . in furture we would like to extend the same across to allow for targeted adversairal guidance using images alone. 

Negative token merging provides a novel direction for performing adversarial guidance directly using visual features from a reference image . This provides a complementary approach to traditionally used negative prompt for adversarial guidance. While performing adversarial guidance using the entire reference image is useful for a range of custom applications (\eg, increasing output diversity, improving output aesthetics, style guidance: Sec.~\ref{sec:experiments}, \ref{sec:analysis} \etc), it may still struggle for applications which require controlled adversarial guidance. Such control can be further useful for applications where the user wants to guide the output but only using certain visual features in the reference image. 

For instance, when performing adversarial guidance for improving diversity, we observe that it improves output diversity for both subject features (\eg, appearance, pose, position, scaling) as well as background features (\eg, time of day, background appearance \etc). In future, we would also like to allow applications where the user can control the visual features across which adversarial guidance is required.

While we provide an initial solution to this via masked adversarial guidance (refer Sec.~\ref{sec:method} of the main paper), controlled guidance is mainly possible for distinct entities (\eg, main subject vs background). In future, we would also like to extend our approach where controlled guidance is possible for attributes (\eg, pose, scale) of the same object. Using multiple reference images for obtaining disentangled control presents as an interesting future direction. However, the same is out-of-scope of the current work and we leave the same here as a direction for future research.
